# Supplementary material for: Applications And Potentials Of Intelligent Swarms For Magnetospheric Studies
Source: arXiv:2107.01601 source file (2021-07-04)
Supplement: Supplementary file 1 [file 9_appendices.tex]

\newpage
\appendix
